# Supplementary material for: Complete asymptotic type-token relationship for growing complex systems with inverse power-law count rankings
Source: arXiv:2511.02069 source file (2026-03-30)
Supplement: Supplementary file 1 [file simple-derivation-of-the-finite-type-token-law.appendix.tex]

\section{Alternative derivation of Heaps' law}
\label{app:simple-type-token.alternative-heaps}

Here we show that, under certain conditions, Heaps’ law naturally arises from a probabilistic argument applied to a sample drawn from a system whose type-size distribution follows a power law,
\begin{equation}
\label{eq:simple-type-token.size-frequency}
    P[l_i = l] \sim l^{-\Omega},
\end{equation}
where $ l_i $ denotes the size (or frequency) of the $ i $-th type, and we restrict our analysis to $\Omega < 2$.

Consider a large reservoir containing $ N_\mathrm{res} $ types and $ L_\mathrm{res} $ total tokens, with type sizes distributed according to Eq.~\eqref{eq:simple-type-token.size-frequency}.  
The reservoir can be interpreted as a language, while the sample represents a text drawn from it.

We now draw elements sequentially from the reservoir and study how the number of distinct types grows with the number of sampled tokens. The probability that the $L$-th sampled element corresponds to a new type is
\begin{equation}
    p(L) = \sum_{i=1}^{N_\mathrm{res}} \frac{l_i}{L_\mathrm{res}} \left( 1-\frac{l_i}{L_\mathrm{res}}\right)^{L-1},
\end{equation}
with $ p(1) = 1 $.

Since $ l_i/L_\mathrm{res} \ll 1 $ and $ L/L_\mathrm{res} \ll 1 $, we can apply a Taylor (binomial) expansion and use the approximation $ \ln(1-x) \simeq -x $ for $ x \ll 1 $. This yields
\begin{equation}
     \left( 1-\frac{l_i}{L_\mathrm{res}}\right)^{L-1} \simeq e^{-(L-1)\frac{l_i}{L_\mathrm{res}}} \simeq e^{-L \frac{l_i}{L_\mathrm{res}}} \simeq e^{l_i \ln \left(1-\frac{L}{L_\mathrm{res}}\right)}
     = \left(1-\frac{L}{L_\mathrm{res}}\right)^{l_i}.
\end{equation}
Therefore,
\begin{equation}
    p(L) \simeq \sum_{i=1}^{N_\mathrm{res}} \frac{l_i}{L_\mathrm{res}} \left(1-\frac{L}{L_\mathrm{res}}\right)^{l_i} 
    = \sum_{l = 1}^{L_\mathrm{res}} \frac{l n_l}{L_\mathrm{res}} \left(1-\frac{L}{L_\mathrm{res}}\right)^l,
    \label{eq:simple-type-token.pksimp}
\end{equation}
where we have transformed the sum over individual elements into a sum over sizes, and $ n_l $ denotes the number of types of size $ l $ in the reservoir.

From Eq.~\eqref{eq:simple-type-token.size-frequency}, we know that $ n_l \sim l^{-\Omega} $.  
Moreover, since $ 1 - \Omega > -1 $ and $ L/L_\mathrm{res} \ll 1 $, the dominant contribution to the sum comes from large $ l $ values. Thus, we can approximate the sum by an integral:
\begin{equation}
    p(L) \sim \int_0^{\infty} \left( 1-\frac{L}{L_\mathrm{res}} \right)^l l^{1-\Omega} \mathrm{d}l \sim L^{\Omega -2},
    \label{eq:simple-type-token.pkscaling}
\end{equation}
and consequently, the expected number of distinct types after $ L $ samples is
\begin{equation}
    N(L) = \sum_{L' = 0}^{L} p(L') \sim \sum_{L' = 0}^{L} (L')^{\Omega-2} \sim L^{\Omega-1}.
    \label{eq:simple-type-token.heaps}
\end{equation}

Finally, note that the exponents in Eqs.~\eqref{eq:simple-type-token.Srt-base-equation} and \eqref{eq:simple-type-token.size-frequency} are related\footnote{Recall that a power-law size distribution $ P(k) \sim k^{-\Omega} $ implies a complementary cumulative distribution
$
P_{>}(k) = \int_{s=k}^{\infty} P(s)\, \mathrm{d}s \sim k^{-\Omega+1}.
$
For a system with $ N $ elements, $ N P_{>}(k) $ gives the number of types with size greater than or equal to $ k $. Identifying this with the rank $ r $ of the type of size $ S_r $, we find
$
r \simeq N P_{>}(S_r) \sim N S_r^{-\Omega+1}.
$
Since $ S_r \sim r^{-\rankdistexponent} $, it follows that $ \Omega = 1 + 1/\rankdistexponent $.} by $\Omega = 1 + 1/\rankdistexponent.$  
Therefore, Eq.~\eqref{eq:simple-type-token.heaps} directly yields Heaps’ law.
